# Supplementary material for: Non-adiabatic exciton-phonon coupling in Raman spectroscopy of layered materials
Source: arXiv:1904.00480 source file (2020-07-31)
Supplement: Supplementary file 1 [file supplementary.pdf]

# Non-adiabatic exciton-phonon coupling in Raman spectroscopy of layered materials – Supplementary Material

Sven Reichardt<sup>1</sup> and Ludger Wirtz<sup>1</sup>

<sup>1</sup>*Department of Physics and Materials Science, University of Luxembourg, 1511 Luxembourg, Luxembourg*

The Supplementary Material is structured as follows:

In Section S1, we provide additional theoretical details of our approach. Section S2 contains supplementary information on the calculation for bulk hexagonal boron nitride (hBN). Finally, we present supplementary material for the calculation for monolayer molybdenum disulfide (MoS<sub>2</sub>) in Section S3.

## S1. THEORETICAL DETAILS

Here we provide more details on how to obtain Eq. (3) from Eq. (2) of the main text within the specified approximations.

First, we expand the (bare) electronic current density and force operators in the basis of Kohn-Sham states:

$$\hat{J}_\mu \equiv \sum_{\mathbf{k}, a, a'} \left( d_{\mathbf{k}, a', a}^{\mu, (b)} \right)^* \hat{c}_{\mathbf{k}, a}^\dagger \hat{c}_{\mathbf{k}, a'} \quad (\text{S1})$$

$$\hat{F}_\lambda \equiv \sum_{\mathbf{k}, b, b'} \left( g_{\mathbf{k}, b', b}^{\lambda, (b)} \right)^* \hat{c}_{\mathbf{k}, b}^\dagger \hat{c}_{\mathbf{k}, b'} \quad (\text{S2})$$

The expansion coefficients are defined such that they denote the matrix elements for *photon/phonon emission*, i.e., *current density/force annihilation*. Note that at zero momentum transfer and for real polarization vectors/phonon eigenvectors, the matrix elements obey  $m_{\mathbf{k}, a', a}^{(b)} = \left( m_{\mathbf{k}, a, a'}^{(b)} \right)^*$ .

In terms of these matrix elements, the time-ordered force-current-current correlation function reads

$$\begin{aligned} \langle 0 | \mathcal{T} \left[ \hat{F}_\lambda(t') \hat{J}_\nu(t) \hat{J}_\mu^\dagger(0) \right] | 0 \rangle_{\text{connect.}} &= \sum_{\mathbf{k}, \mathbf{k}', \mathbf{k}''} \sum_{\substack{a, b, c \\ a', b', c'}} \left( g_{\mathbf{k}, a', a}^{\lambda, (b)} \right)^* \left( d_{\mathbf{k}', b', b}^{\nu, (b)} \right)^* d_{\mathbf{k}'', c, c'}^{\mu, (b)} \\ &\times \langle 0 | \mathcal{T} \left[ \hat{c}_{\mathbf{k}, a}^\dagger(t') \hat{c}_{\mathbf{k}, a'}(t') \hat{c}_{\mathbf{k}', b}^\dagger(t) \hat{c}_{\mathbf{k}', b'}(t) \hat{c}_{\mathbf{k}'', c}^\dagger(0) \hat{c}_{\mathbf{k}'', c'}(0) \right] | 0 \rangle_{\text{connect.}}. \end{aligned} \quad (\text{S3})$$

The last factor is the fully connected part of the three-particle Green's function. We approximate it in a controlled way with the help of Feynman diagrams, as shown in Fig. S1. The first term shown corresponds to the independent-particle

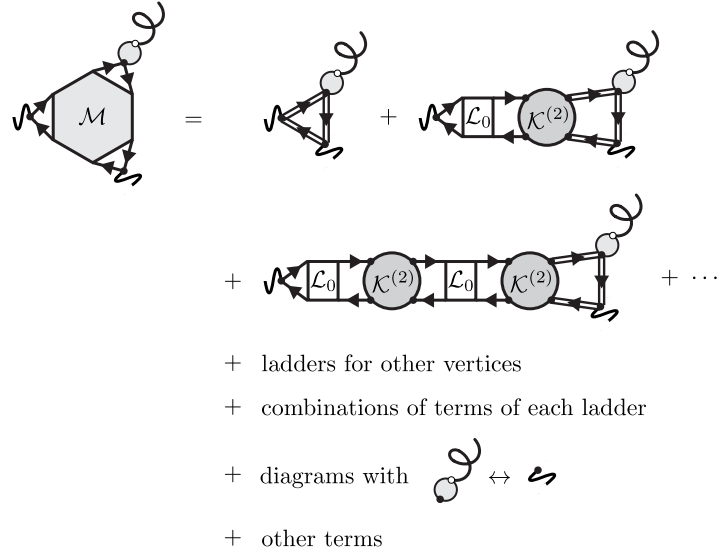

FIG. S1. **Diagrammatic analysis of the reduced matrix element.** Dark dots (light circles) denote the bare electron-photon (-phonon) vertex. Double lines denote the one-electron Green's function.  $\mathcal{L}$  ( $\mathcal{L}_0$ ) and  $\mathcal{K}^{(2)}$  denote the interacting (independent-particle) two-particle correlation function and two-particle interaction kernel, respectively.

approximation to the three-particle correlation function. In the second term, we include the first-order correction to the electron-incoming photon vertex due to two-particle inter-electron interactions. We denote the kernel describing the latter by  $\mathcal{K}^{(2)}$ , while  $\mathcal{L}_0$  represents the two-particle correlation function on the independent-particle level. The second line shows the second-order correction to the same vertex while the dots refer to higher-order corrections of the same form. We consider the same summation of terms for all three vertices simultaneously. In order to consider all topologically distinct diagrams, we also need to consider terms in which the fermion flow is reversed, i.e., in which the vertices for the outgoing photon and phonon are interchanged.

The *ladder-like approximation* introduced in the main text now consists of neglecting all other terms that do not follow the ladder-like structure depicted in the first two lines of Fig. S1. As shown in Fig. 1 of the main text, the

summation of terms at each vertex can be carried out separately. The double Fourier transform of the force-current-current correlation function, which up to a factor of  $i$  corresponds to the reduced matrix element, then takes on the form

$$i\tilde{\mathcal{M}}_{\mu\nu}^{\lambda}(\omega', \omega) = \sum_{\mathbf{k}} \sum_{\substack{a,b,c \\ a',b',c'}} \bar{g}_{\mathbf{k},a',a}^{\lambda}(\omega') \bar{d}_{\mathbf{k},b',b}^{\nu}(\omega) d_{\mathbf{k},c,c'}^{\mu}(\omega + \omega') \\ \times \frac{1}{\hbar^2} \int_{-\infty}^{+\infty} dt e^{i\omega t} \int_{-\infty}^{+\infty} dt' e^{i\omega' t'} \langle 0 | \mathcal{T} \left[ \hat{c}_{\mathbf{k},a}^{\dagger}(t') \hat{c}_{\mathbf{k},a'}(t') \hat{c}_{\mathbf{k},b}^{\dagger}(t) \hat{c}_{\mathbf{k},b'}(t) \hat{c}_{\mathbf{k},c}^{\dagger}(0) \hat{c}_{\mathbf{k},c'}(0) \right] | 0 \rangle \Big|_{\text{IP,connect.}}, \quad (\text{S4})$$

where the three-particle correlation function now only appears in the form of its independent-particle version. The first three factors denote the Fourier transforms of the *exact* vertices, with a bar denoting the vertices for photon/phonon emission. To obtain concrete expressions for the latter, we approximate the two-particle interaction kernel as mentioned in the main text.

In the case of the electron-light vertex, we approximate it as the sum of a statically screened, attractive electron-hole Coulomb interaction and a bare, repulsive exchange part. We can then give an explicit expression for the Fourier-transformed vertex function by making use of the Bethe-Salpeter equation

$$L_{\mathbf{k},a',a}(\omega) = L_{0;\mathbf{k},a',a}(\omega) \delta_{\mathbf{k},\mathbf{k}'} \delta_{a',b'} \delta_{a,b} + L_{0;\mathbf{k},a',a}(\omega) \sum_{\mathbf{k}''} \sum_{c',c} K_{\mathbf{k},a',a}^{(2)} L_{\mathbf{k}'',c',c}(\omega) L_{\mathbf{k}',b',b}(\omega) \quad (\text{S5})$$

where we now use non-calligraphic script to denote the approximated quantities. Note that we also use the quasi-particle approximation for  $L_0$ , so that it only depends on two band indices. As shown in Fig. 1 of the main text, we can identify the right-hand side up to a factor of  $L_0$  as the factor that modulates the bare vertex, and we thus have

$$d_{\mathbf{k},a',a}^{\mu}(\omega) = d_{\mathbf{k},a',a}^{\mu,(b)} + \sum_{\mathbf{k}',\mathbf{k}''} \sum_{\substack{b',c' \\ b,c}} K_{\mathbf{k},a',a}^{(2)} L_{\mathbf{k}',b',b}(\omega) d_{\mathbf{k}'',c',c}^{\mu,(b)} = L_{0;\mathbf{k},a',a}^{-1}(\omega) \sum_{\mathbf{k}'} \sum_{b',b} L_{\mathbf{k},a',a}(\omega) d_{\mathbf{k}',b',b}^{\mu,(b)} \quad (\text{S6})$$

for photon *absorption* and

$$\bar{d}_{\mathbf{k},a',a}^{\mu}(\omega) = \left( d_{\mathbf{k},a',a}^{\mu,(b)} \right)^* + \sum_{\mathbf{k}',\mathbf{k}''} \sum_{\substack{b',c' \\ b,c}} \left( d_{\mathbf{k}',b',b}^{\mu,(b)} \right)^* L_{\mathbf{k}'',c',c}(\omega) K_{\mathbf{k},a',a}^{(2)} = \sum_{\mathbf{k}'} \sum_{b',b} \left( d_{\mathbf{k}',b',b}^{\mu,(b)} \right)^* L_{\mathbf{k}',b',b}(\omega) L_{0;\mathbf{k},a',a}^{-1}(\omega). \quad (\text{S7})$$

for photon *emission*. Lastly, as mentioned in the main text, we also use the *Tamm-Dancoff approximation*, which is justified for the semiconducting systems discussed in the main text. In this approximation, the independent-particle two-particle correlation function reads

$$L_{0;\mathbf{k},a',a}(\omega) = \frac{\bar{f}_{\mathbf{k},a'} f_{\mathbf{k},a}}{\hbar\omega - (\varepsilon_{\mathbf{k},a'} - \varepsilon_{\mathbf{k},a}) + i\eta} + \frac{f_{\mathbf{k},a'} \bar{f}_{\mathbf{k},a}}{-\hbar\omega - (\varepsilon_{\mathbf{k},a} - \varepsilon_{\mathbf{k},a'}) + i\eta}, \quad (\text{S8})$$

where  $f_{\mathbf{k},a}$  denotes the occupancy of the state  $|\mathbf{k}, a\rangle$  in the ground state,  $\bar{f}_{\mathbf{k},a} \equiv 1 - f_{\mathbf{k},a}$ , and  $\eta$  is a positive infinitesimal. The interacting two-particle correlation function can be expressed in terms of the excitonic wave functions  $A_{\mathbf{k},a',a}^S$  and energies  $E_S$  as

$$L_{\mathbf{k},a',a}(\omega) = \sum_S \left[ \bar{f}_{\mathbf{k},a'} f_{\mathbf{k},a} \bar{f}_{\mathbf{k}',b'} f_{\mathbf{k}',b} \frac{A_{\mathbf{k},a',a}^S (A_{\mathbf{k}',b',b}^S)^*}{\hbar\omega - E_S + i\eta} + f_{\mathbf{k},a'} \bar{f}_{\mathbf{k},a} f_{\mathbf{k}',b'} \bar{f}_{\mathbf{k}',b} \frac{(A_{\mathbf{k},a,a'}^S)^* A_{\mathbf{k}',b',b}^S}{-\hbar\omega - E_S + i\eta} \right], \quad (\text{S9})$$

where the sum runs over all *positive-energy* excitons. Note that within the Tamm-Dancoff approximation, an excitonic envelope wave function  $A_{\mathbf{k},a',a}^S$  for positive-energy excitons has non-vanishing components only for  $a' \in \mathcal{C}$  and  $a \in \mathcal{V}$ , where  $\mathcal{C}$  and  $\mathcal{V}$  denote the sets of conduction and valence band indices, respectively. Combining the last three equations, we arrive at the final expression we use to approximate the exact electron-photon vertices:

$$d_{\mathbf{k},a',a}^{\mu}(\omega) = \sum_S \left[ \bar{f}_{\mathbf{k},a'} f_{\mathbf{k},a} A_{\mathbf{k},a',a}^S \frac{\hbar\omega - (\varepsilon_{\mathbf{k},a'} - \varepsilon_{\mathbf{k},a}) + i\eta}{\hbar\omega - E_S + i\eta} d_S^{\mu} \right. \\ \left. + f_{\mathbf{k},a'} \bar{f}_{\mathbf{k},a} (A_{\mathbf{k},a,a'}^S)^* \frac{-\hbar\omega - (\varepsilon_{\mathbf{k},a} - \varepsilon_{\mathbf{k},a'}) + i\eta}{-\hbar\omega - E_S + i\eta} (d_S^{\mu})^* \right] \quad (\text{S10})$$

and

$$\begin{aligned} \bar{d}_{\mathbf{k},a',a}^\mu(\omega) = \sum_S \left[ \bar{f}_{\mathbf{k},a'} f_{\mathbf{k},a} (d_S^\mu)^* \frac{\hbar\omega - (\varepsilon_{\mathbf{k},a'} - \varepsilon_{\mathbf{k},a}) + i\eta}{\hbar\omega - E_S + i\eta} (A_{\mathbf{k},a',a}^S)^* \right. \\ \left. + f_{\mathbf{k},a'} \bar{f}_{\mathbf{k},a} d_S^\mu \frac{-\hbar\omega - (\varepsilon_{\mathbf{k},a} - \varepsilon_{\mathbf{k},a'}) + i\eta}{-\hbar\omega - E_S + i\eta} A_{\mathbf{k},a,a'}^S \right], \end{aligned} \quad (\text{S11})$$

with  $d_S^\mu$  as defined in Eq. (4) of the main text.

For the exact electron-phonon vertex, we follow the same line of argument, but approximate the two-particle interaction kernel in that case with the kernel corresponding to time-dependent density functional theory. As shown in Ref. [23], this approximation is exactly equivalent to using the statically screened electron-phonon coupling on the level of density functional perturbation theory. In addition, we also neglect the frequency dependence of the vertex function, i.e., we use

$$\bar{g}_{\mathbf{k},a',a}^\lambda(\omega) \rightarrow (g_{\mathbf{k},a',a}^\lambda)^*|_{\text{DFPT}}, \quad (\text{S12})$$

which is justified for systems with a band gap much larger than the phonon frequency. Note, however, that we *do retain the phonon frequency-dependence of the three-particle independent-particle correlation function* as there the frequency of the photon needs to be considered as well, which reduces the effective band gap seen by the phonon in the three-particle correlation function.

Finally, we also give the explicit form of the Fourier transformed independent-particle three-particle correlation function. Treating it on the level of the quasi-particle approximation, one finds

$$\begin{aligned} & \frac{1}{\hbar^2} \int_{-\infty}^{+\infty} dt e^{i\omega t} \int_{-\infty}^{+\infty} dt' e^{i\omega' t'} \langle 0 | \mathcal{T} \left[ \hat{c}_{\mathbf{k},a}^\dagger(t') \hat{c}_{\mathbf{k},a'}(t') \hat{c}_{\mathbf{k},b}^\dagger(t) \hat{c}_{\mathbf{k},b'}(t) \hat{c}_{\mathbf{k},c}^\dagger(0) \hat{c}_{\mathbf{k},c'}(0) \right] | 0 \rangle \Big|_{\text{IP,connect.}} \\ &= \frac{1}{\hbar^2} \int_{-\infty}^{+\infty} dt e^{i\omega t} \int_{-\infty}^{+\infty} dt' e^{i\omega' t'} (-1) \\ & \quad \times \left\{ \delta_{a',b} \delta_{b',c} \delta_{c',a} \langle 0 | \mathcal{T} \left[ \hat{c}_{\mathbf{k},a}(t') \hat{c}_{\mathbf{k},a}^\dagger(t) \right] | 0 \rangle \langle 0 | \mathcal{T} \left[ \hat{c}_{\mathbf{k},b}(t) \hat{c}_{\mathbf{k},b}^\dagger(0) \right] | 0 \rangle \langle 0 | \mathcal{T} \left[ \hat{c}_{\mathbf{k},c}(0) \hat{c}_{\mathbf{k},c}^\dagger(t') \right] | 0 \rangle \right. \\ & \quad \left. + \delta_{a',c} \delta_{c',b} \delta_{b',a} \langle 0 | \mathcal{T} \left[ \hat{c}_{\mathbf{k},a}(t') \hat{c}_{\mathbf{k},a}^\dagger(0) \right] | 0 \rangle \langle 0 | \mathcal{T} \left[ \hat{c}_{\mathbf{k},b}(t) \hat{c}_{\mathbf{k},b}^\dagger(t') \right] | 0 \rangle \langle 0 | \mathcal{T} \left[ \hat{c}_{\mathbf{k},c}(0) \hat{c}_{\mathbf{k},c}^\dagger(t) \right] | 0 \rangle \right\} \\ & \equiv i \delta_{a',b} \delta_{b',c} \delta_{c',a} R_{0;\mathbf{k},c,a,b}(-\omega', -\omega) + i \delta_{a',c} \delta_{c',b} \delta_{b',a} R_{0;\mathbf{k},a,b,c}(\omega', \omega). \end{aligned} \quad (\text{S13})$$

In the last step, we identified the Fourier transform of the independent-particle three-particle correlation function on the quasi-particle level, which is explicitly given by

$$\begin{aligned} & (-i) R_{0;\mathbf{k},a,b,c}(\omega_1, \omega_2) \\ &= \frac{1}{\hbar^2} \int_{-\infty}^{+\infty} dt e^{i\omega t} \int_{-\infty}^{+\infty} dt' e^{i\omega' t'} \langle 0 | \mathcal{T} \left[ \hat{c}_{\mathbf{k},a}(t') \hat{c}_{\mathbf{k},a}^\dagger(0) \right] | 0 \rangle \langle 0 | \mathcal{T} \left[ \hat{c}_{\mathbf{k},b}(t) \hat{c}_{\mathbf{k},b}^\dagger(t') \right] | 0 \rangle \langle 0 | \mathcal{T} \left[ \hat{c}_{\mathbf{k},c}(0) \hat{c}_{\mathbf{k},c}^\dagger(t) \right] | 0 \rangle \\ &= + \frac{f_{\mathbf{k},a} \bar{f}_{\mathbf{k},b} \bar{f}_{\mathbf{k},c}}{[-\hbar\omega_1 - \hbar\omega_2 - (\varepsilon_{\mathbf{k},c} - \varepsilon_{\mathbf{k},a}) + i\eta][-\hbar\omega_1 - (\varepsilon_{\mathbf{k},b} - \varepsilon_{\mathbf{k},a}) + i\eta]} \\ & \quad - \frac{\bar{f}_{\mathbf{k},a} f_{\mathbf{k},b} f_{\mathbf{k},c}}{[\hbar\omega_1 + \hbar\omega_2 - (\varepsilon_{\mathbf{k},a} - \varepsilon_{\mathbf{k},c}) + i\eta][\hbar\omega_1 - (\varepsilon_{\mathbf{k},a} - \varepsilon_{\mathbf{k},b}) + i\eta]} \\ & \quad + \frac{\bar{f}_{\mathbf{k},a} \bar{f}_{\mathbf{k},b} f_{\mathbf{k},c}}{[\hbar\omega_1 + \hbar\omega_2 - (\varepsilon_{\mathbf{k},a} - \varepsilon_{\mathbf{k},c}) + i\eta][\hbar\omega_2 - (\varepsilon_{\mathbf{k},b} - \varepsilon_{\mathbf{k},c}) + i\eta]} \\ & \quad - \frac{f_{\mathbf{k},a} f_{\mathbf{k},b} \bar{f}_{\mathbf{k},c}}{[-\hbar\omega_1 - \hbar\omega_2 - (\varepsilon_{\mathbf{k},c} - \varepsilon_{\mathbf{k},a}) + i\eta][-\hbar\omega_2 - (\varepsilon_{\mathbf{k},c} - \varepsilon_{\mathbf{k},b}) + i\eta]} \\ & \quad + \frac{\bar{f}_{\mathbf{k},a} f_{\mathbf{k},b} \bar{f}_{\mathbf{k},c}}{[\hbar\omega_1 - (\varepsilon_{\mathbf{k},a} - \varepsilon_{\mathbf{k},b}) + i\eta][-\hbar\omega_2 - (\varepsilon_{\mathbf{k},c} - \varepsilon_{\mathbf{k},b}) + i\eta]} \\ & \quad - \frac{f_{\mathbf{k},a} \bar{f}_{\mathbf{k},b} f_{\mathbf{k},c}}{[-\hbar\omega_1 - (\varepsilon_{\mathbf{k},b} - \varepsilon_{\mathbf{k},a}) + i\eta][\hbar\omega_2 - (\varepsilon_{\mathbf{k},b} - \varepsilon_{\mathbf{k},c}) + i\eta]}. \end{aligned} \quad (\text{S14})$$

It is then straightforward to obtain Eqs. (3-5) from the main text by combining all of the individual pieces and replacing  $\eta$  by the electronic broadening  $\gamma$ .

## S2. SUPPLEMENTARY INFORMATION FOR THE HBN CALCULATION

In this section, we provide more computational details for the calculations for bulk hexagonal boron nitride. We show the electronic band structure and plots of the excitonic envelope wave functions in reciprocal space for the first four optically active excitons. Finally, we discuss how the calculated Raman intensity in both the non-adiabatic and adiabatic cases changes when only inter- or intra-exciton scattering is taken into account.

### Computational details

The ground state properties of bulk hexagonal boron nitride in the  $AA'$  stacking configuration were computed on the level of density functional theory (DFT) within the local density approximation (LDA) for the exchange-correlation functional in the parametrization due to Perdew and Zunger [34]. All DFT calculations were performed with the `PWscf` code of the `QuantumESPRESSO` suite [33] using norm-conserving, non-relativistic, core-corrected pseudopotentials. We use a plane-wave basis set with an energy cutoff of 110 Ry for the electronic wave functions and 440 Ry for the charge density. For integrations over the first Brillouin zone, a uniform  $\mathbf{k}$ -point mesh of size  $12 \times 12 \times 2$  was used. The lattice parameters were relaxed prior to the calculation, yielding values of  $a=2.478$  Å and  $c=6.453$  Å for the in- and out-of-plane lattice constants, respectively. For the electronic excited state properties, we computed the electronic band structure on a  $36 \times 36 \times 2$   $\mathbf{k}$ -point mesh for 200 (spin-degenerate) bands.

The calculation of the excitonic eigenenergies and envelope wave functions was performed with the `yambo` code [35]. The two-particle interaction kernel was computed on the level of the Tamm-Dancoff approximation as the sum of a statically screened, attractive Coulomb part plus a repulsive, bare exchange part. The static inverse dielectric screening function was computed on the level of the random phase approximation using plane-wave cutoffs of 60 Ry each for the electronic wave functions and the dielectric response function in reciprocal space. For the calculation of the actual two-particle interaction kernel, we truncated the attractive screened Coulomb part at a plane-wave energy cutoff of 10 Ry and the repulsive bare exchange part at a plane-wave cutoff of 20 Ry. We included the upper two valence and lower two conduction bands in the construction of the two-particle interaction kernel. A rigid band energy shift of 2 eV was added to all independent-particle transition energies in order to account for the underestimation of the band gap in DFT. This value was obtained in previous first-principles calculations on the level of the  $GW$  approximation [20]. Finally, we solve the Bethe-Salpeter equation iteratively for the first 2000 excitonic eigenenergies and envelope wave functions using the `SLEPc` library [36].

For the screened electron-phonon coupling, we approximate the two-particle interaction kernel on the level of time-dependent density functional theory. As this approximation is equivalent to obtaining the screened electron-phonon matrix elements with density functional perturbation theory [23], we calculate the screened matrix elements with the `PH` code of the `QuantumESPRESSO` suite [33]. Lastly, for the phonon frequency of the degenerate, Raman-active in-plane optical mode ( $E_{2g}$ -symmetry), we use the calculated value of  $1388.6 \text{ cm}^{-1}$ .

## Electronic band structure

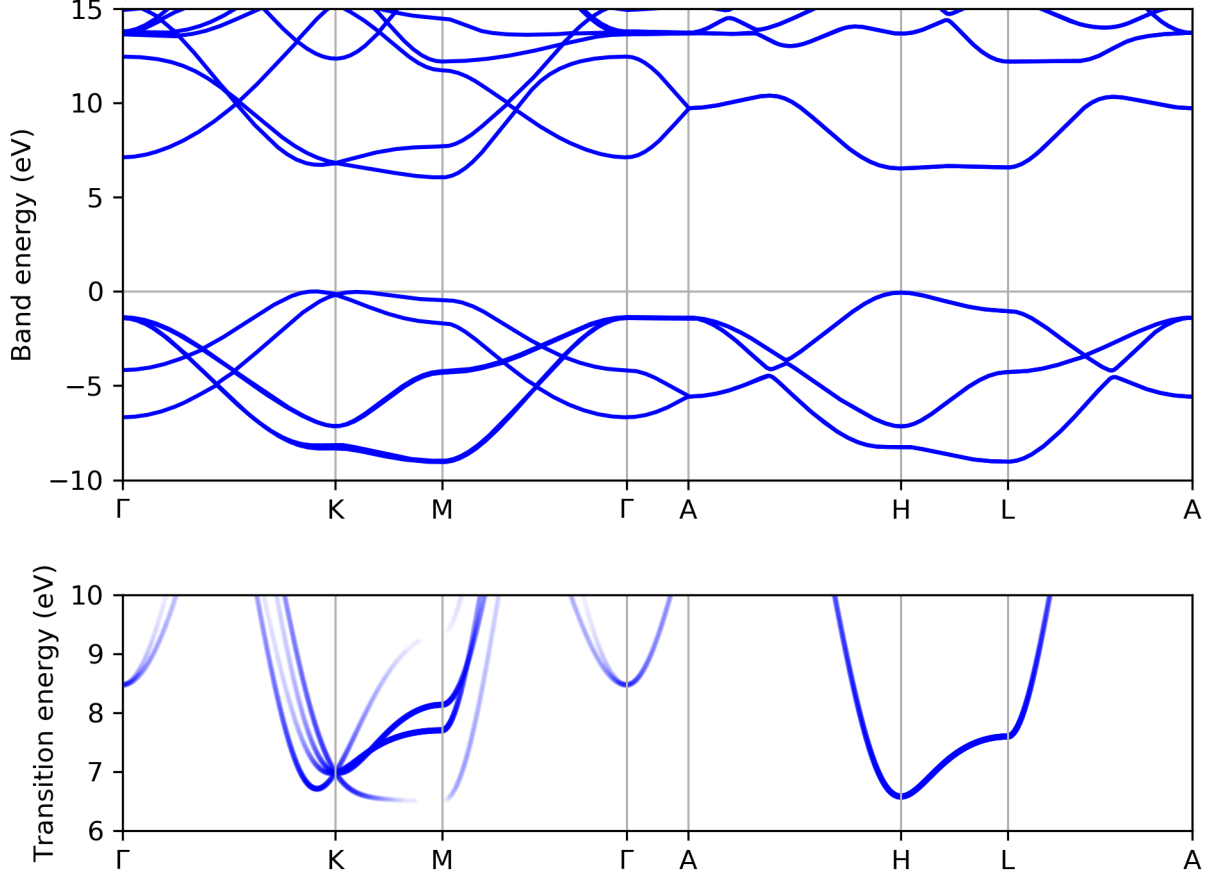

FIG. S2. **hBN: Electronic (transition) band structure.** Top: Electronic band structure on the level of Kohn-Sham DFT within the LDA. A rigid shift of 2 eV was added to all conduction band energies. Bottom: Electronic transition band structure obtained from the electronic band structure. The opacity of the lines corresponds to the optical activity of the transition.

The electronic band structure of bulk hexagonal boron nitride is shown in Fig. S2. We show both the electronic band structure on the level of Kohn-Sham DFT on the LDA level (top panel) and the resulting transition band structure weighted by the absolute value of the in-plane polarization-averaged transition dipole matrix element squared (bottom panel). As mentioned in the previous section, we shifted all conduction bands by 2 eV to account for the underestimation of the band gap in DFT [20].

The band structure is characterized by an indirect gap of 6.038 eV between the top of the valence band near the  $K$ -point and the bottom of the conduction band at the  $M$ -point. The direct gap of 6.500 eV is located at  $M$  and is quasi-degenerate with the transition at  $H$ . The low-energy electronic transitions are located around the  $M$ -,  $H$ -, and  $K$ -points as well as on the line  $K$ - $M$ .

Near the band gap, i.e., in the vicinity of the  $M$ - and  $H$ -points, the electronic transitions are either only weakly optically inactive ( $M$ -point) or the band structure is circularly symmetric ( $H$ -point). In case of the former the respective transitions are trivially prevented from participating in the Raman scattering process. In case of the latter, the full rotation symmetry leads to full angular momentum conservation, which in turn suppresses scattering involving the degenerate, vector-like  $E_{2g}$ -phonon, as argued in the main text. This explains the absence of a sizable Raman intensity near the band edge on the independent-particle level.

For the exciton physics, the most important region is the immediate neighborhood of the  $K$ -point, as the overtone excitons are mostly composed of transitions from there. Close to  $K$ , the low-energy transition band structure is circularly symmetric, i.e., for the physics that involves only these transitions, the system again behaves as if it possessed full rotation symmetry. This argument is used in the main text when the principle of angular momentum conservation is invoked to discuss the suppression of the Raman intensity for the overtone excitons. A bit further

away from  $K$ , the valley along the  $\Gamma$ - $K$  direction breaks the full rotation symmetry, which allows the excitons that are more delocalized in  $\mathbf{k}$ -space to contribute to the Raman scattering process.

## Excitonic envelope wave functions

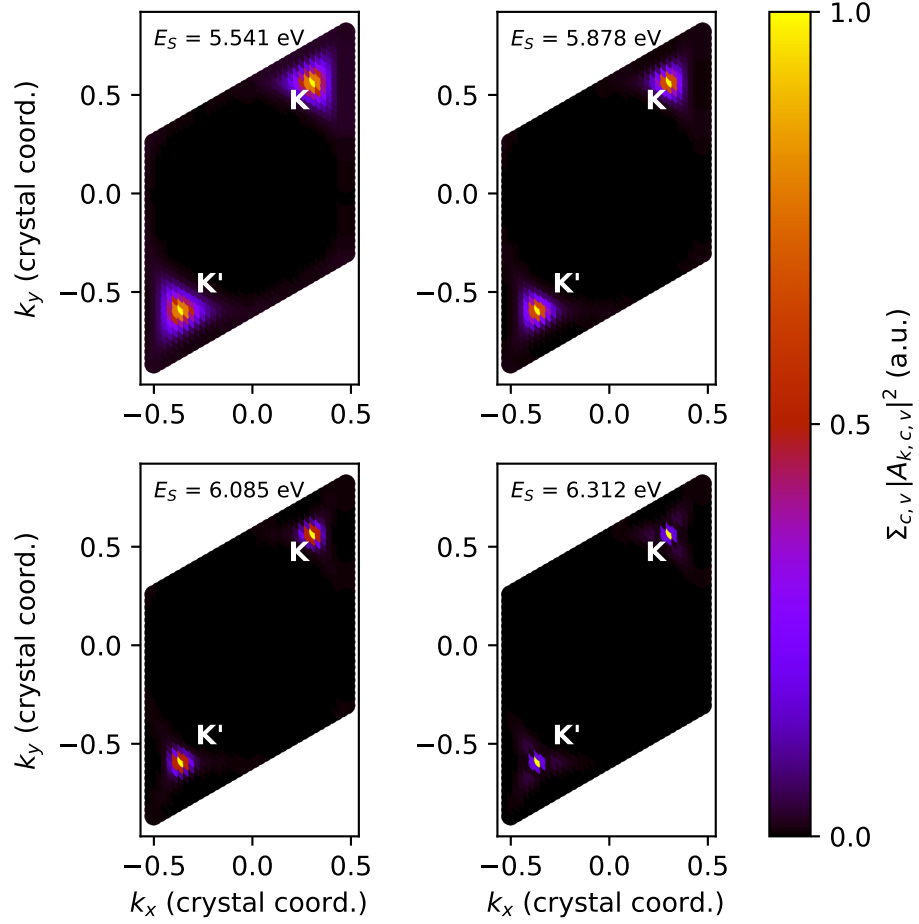

FIG. S3. **hBN: Exciton envelope wave functions in reciprocal space.** Each panel shows the band-summed square of the envelope wave function  $|A_{\mathbf{k},c,v}^S|^2$  as a function of the wave vector  $\mathbf{k}$  in the plane containing the  $\Gamma$ - and  $K$ -point. Shown are the wave functions of the first four bright excitons.

In Fig. S3, we show the state-summed envelope wave functions for the first four bright excitons as a function of wave vector  $\mathbf{k}$  in the plane containing the  $\Gamma$ - and  $K$ -point (compare also Ref. [26] for the single-layer case). While the first bright exciton is strongly delocalized in  $\mathbf{k}$ -space, the second one is already more localized around the  $K$ - and  $K'$ -points, although still showing a trigonally warped shape. By contrast, the third and fourth excitons are strongly localized around  $K^{(l)}$  and their wave functions are circularly symmetric. Together with the circularly symmetric band structure around the  $K^{(l)}$ -point, this leads to the system behaving as if it featured almost full rotation symmetry and hence resonant Raman scattering involving a degenerate phonon mode is suppressed on account of angular momentum conservation [6, 13, 29].

Raman intensity with only inter- or intra-exciton scattering

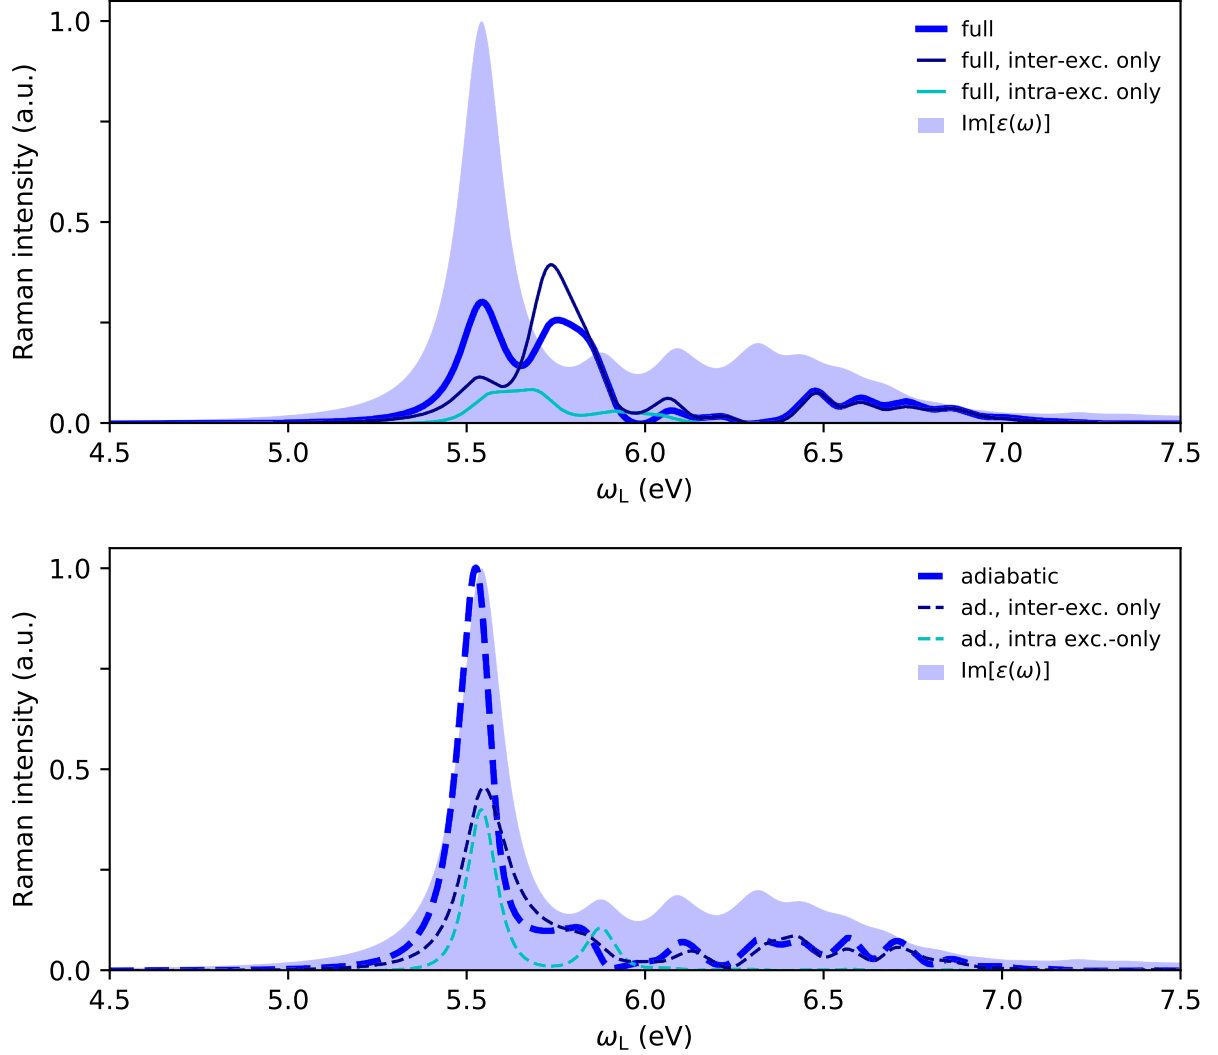

FIG. S4. **hBN: Raman intensity with only inter- or intra-exciton scattering.** Raman intensity with all contributions (thick lines) and with only inter- or intra-exciton scattering (darker and lighter thin lines, respectively) taken into account. Top panel: full, non-adiabatic case. Bottom panel: adiabatic limit. The shaded area represents the absorption spectrum. The Raman intensity is given in the same units in both panels and as in Fig. 2 of the main text.

In order to further demonstrate that the redistribution of oscillator strength from the second to the first bright exciton in the non-adiabatic theory indeed arises from inter-exciton scattering, we calculate the Raman intensity with only these contributions. Note in this context that many of the exciton states are degenerate. For example, the first excitonic resonance in the absorption spectrum is due to a bright exciton doublet of  $E_{2u}$ -symmetry, which is slightly higher in energy than the lowest (dark) exciton doublet of  $E_{2g}$ -symmetry [28]. We thus define a Raman matrix element that only contains *intra*-exciton scattering processes (i.e., from one excitonic state to itself or to a degenerate partner) via the restricted sum

$$\tilde{\mathcal{M}}_{\mu\nu}^{\lambda}|_{\text{intra}}(\omega_L - \omega_D, \omega_D) = \sum_{S,S'} \Big|_{E_S=E_{S'}} \left[ \frac{d_S^{\mu}(g_{S,S'}^{\lambda})^*(d_{S'}^{\nu})^*}{(\hbar\omega_L - E_S + i\gamma)(\hbar\omega_D - E_{S'} + i\gamma)} + \frac{(d_S^{\mu})^* g_{S,S'}^{\lambda} d_{S'}^{\nu}}{(\hbar\omega_L + E_S - i\gamma)(\hbar\omega_D + E_{S'} - i\gamma)} \right]. \quad (\text{S15})$$

We then further define the Raman matrix element with only *inter*-exciton scattering processes as the difference

$$\tilde{\mathcal{M}}_{\mu\nu}^{\lambda}|_{\text{inter}}(\omega_L - \omega_D, \omega_D) \equiv \tilde{\mathcal{M}}_{\mu\nu}^{\lambda}(\omega_L - \omega_D, \omega_D) - \tilde{\mathcal{M}}_{\mu\nu}^{\lambda}|_{\text{intra}}(\omega_L - \omega_D, \omega_D) \quad (\text{S16})$$

of the full Raman matrix element of Eq. (3) of the main text and the intra-exciton-only one from Eq. (S15). The double sum over excitons in Eq. (S15) is understood to run over all exciton states, taking into account all off-diagonal exciton-phonon matrix elements between degenerate states, but ignoring the coupling of one exciton multiplet to another.

With these two restricted matrix elements, we can compute the Raman intensity again, this time, however, only with intra- or inter-exciton scattering. The resulting intensities are shown in Fig. S4. In the case of the adiabatic limit (bottom panel), intra- (lighter color) and inter-exciton scattering (darker color) contribute to the total Raman intensity with about equal weight and they add up constructively. By contrast, the full non-adiabatic result (top panel) is strongly dominated by the contribution from *inter*-exciton scattering. Moreover, while at the first exciton resonance, inter- and intra-exciton scattering reinforce each other, at the second excitonic resonance, the two contributions destructively interfere. Compared to the adiabatic case, we thus observe that the non-adiabatic contribution from the inter-exciton scattering terms changes sign, which is a typical behavior around a resonance and thus further demonstrates the importance of considering resonant scattering due to the finite phonon frequency.

The importance of inter-exciton scattering can further be illustrated by considering the convergence of the Raman matrix element with the number of exciton multiplets ( $N_{\text{exc}}$ ) included, as shown in Fig. S5. In both the non-adiabatic and adiabatic cases does the inter-exciton scattering contribution to the Raman matrix element (right column) converge much more slowly with  $N_{\text{exc}}$  than the intra-exciton scattering part (center column). This can be attributed to the fact that the intra-exciton scattering contribution involves a sum of almost *double-resonant* amplitudes proportional to  $(\hbar\omega_L - E_S + i\gamma)(\hbar\omega_D - E_S + i\gamma)$ . In this case and for  $\omega_L$  near one of the excitonic resonances, the non-resonant excitons do not contribute at all and this contribution to the Raman intensity is already converged when the resonant exciton is included. By contrast, the inter-exciton scattering part of the Raman matrix element is only *single-resonant* at each exciton energy, since the amplitudes are of the form  $[(\hbar\omega_L - E_S + i\gamma)(\hbar\omega_D - E_{S'} + i\gamma)]^{-1}$ . While each of these amplitudes by itself is smaller in magnitude than the double-resonant contribution, in the sum over all excitons multiplets  $S'$ , these amplitudes still add up to yield a sizable contribution to the total Raman intensity. This implies, however, that many non-resonant excitonic multiplets need to be considered before the inter-exciton part of the Raman intensity converges.

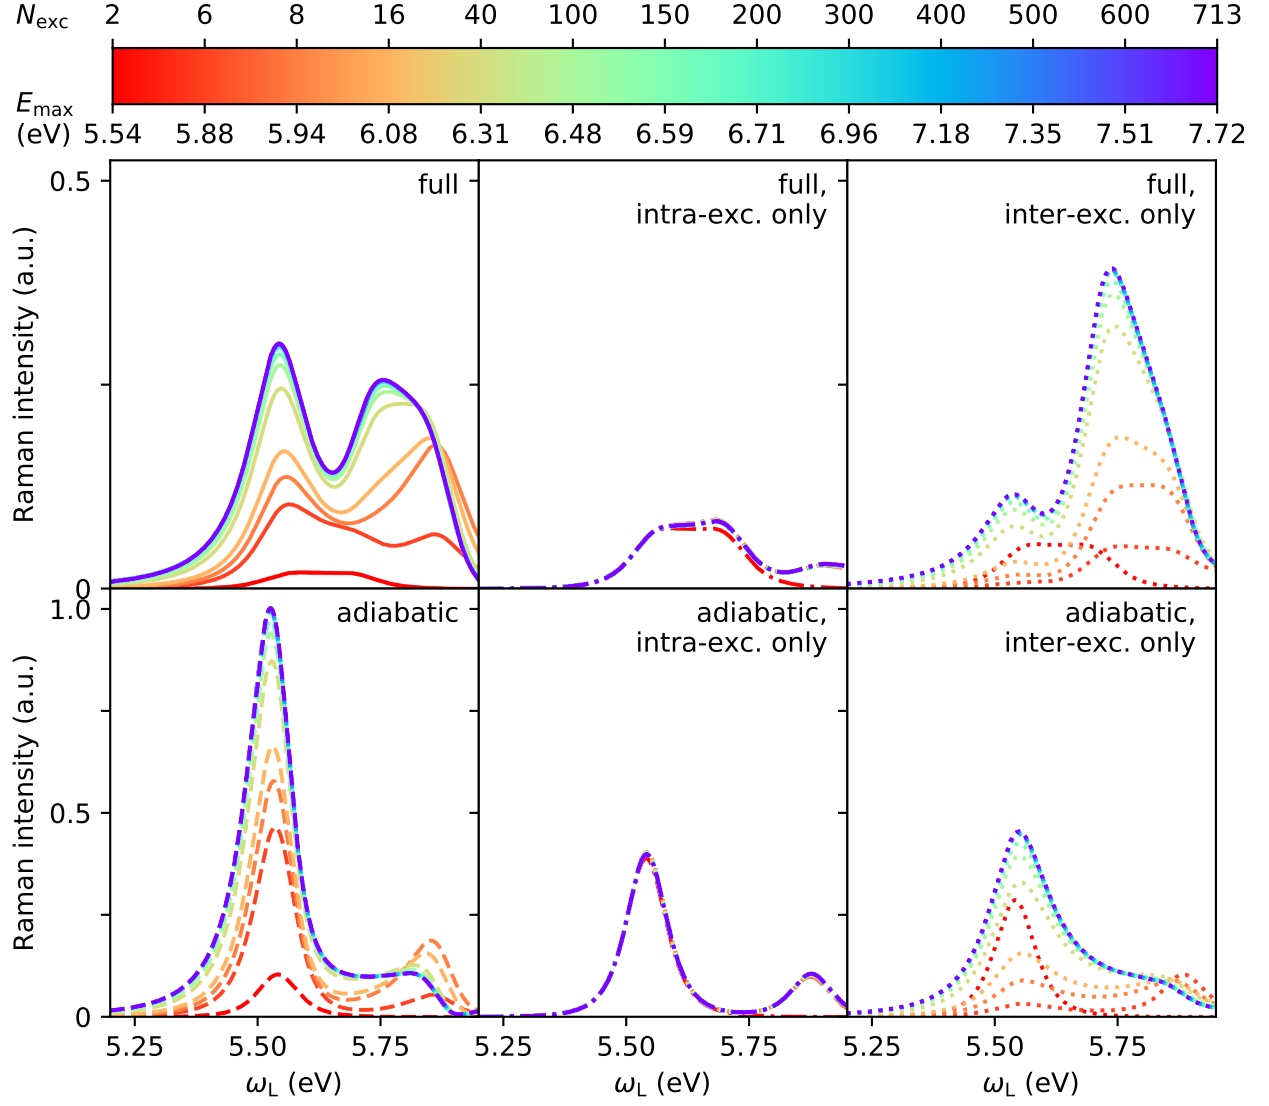

FIG. S5. **hBN: Raman intensity for different numbers of exciton multiplets included.** Raman intensity in the full, non-adiabatic case (top row) and in the adiabatic limit (bottom row) for different numbers of included exciton multiplets. The line color corresponds to the number of included exciton multiplets, with the maximum exciton energy included being indicated below the color bar. The three columns correspond to the Raman intensity with all contributions (left) and with only intra- (center) or inter-exciton (right column) scattering taken into account. The Raman intensity is given in the same units in all the panels and as in Fig. 2 of the main text.

### S3. SUPPLEMENTARY INFORMATION FOR THE $\text{MOS}_2$ CALCULATION

Here we provide more information computational details for the calculations for monolayer molybdenum disulfide. As for boron nitride, we show the excitonic envelope wave functions for the first three optically active excitons and the electronic band structure. Finally, we discuss how the calculated Raman intensity for both the  $E'$ - and  $A'_1$ -mode are differently affected by the contributions from inter- or intra-exciton scattering.

#### Computational details

The ground state properties of monolayer molybdenum disulfide were computed on the level of density functional theory within the local density approximation for the exchange-correlation functional in the parametrization due to Perdew and Zunger [34]. All DFT calculations were performed with the `PWscf` code of the `QuantumESPRESSO` suite [33] using norm-conserving, fully relativistic pseudopotentials for both sulfur and molybdenum to account for the effects of spin-orbit interactions. We use a plane-wave basis set with an energy cutoff of 90 Ry for the electronic wave functions and 360 Ry for the charge density. For integrations over the first Brillouin zone, a uniform  $\mathbf{k}$ -point mesh of size  $12 \times 12 \times 1$  was used. The lattice parameter was relaxed prior to the calculation, yielding a value of  $a=3.170$  Å for the in-plane lattice constant. To preserve the single-layer nature of the system, we use a vacuum spacing of 16 Å between periodic images of the monolayer. For the electronic excited state properties, we computed the electronic band structure on a  $24 \times 24 \times 1$   $\mathbf{k}$ -point mesh with spin-orbit coupling for 400 (in general spin-non-degenerate) bands.

The calculation of the excitonic eigenenergies and envelope wave functions was performed with the `yambo` code [35]. The two-particle interaction kernel was computed on the level of the Tamm-Dancoff approximation as the sum of a statically screened, attractive Coulomb part plus a repulsive, bare exchange part. The static inverse dielectric screening function was computed on the level of the random phase approximation using plane-wave cutoffs of 60 Ry each for the electronic wave functions and the dielectric response function in reciprocal space. For the calculation of the actual two-particle interaction kernel, we truncated the attractive screened Coulomb part at a plane-wave energy cutoff of 10 Ry and the repulsive bare exchange part at a plane-wave cutoff of 20 Ry. We included the upper eight valence and lower eight conduction bands in the construction of the two-particle interaction kernel. A rigid band energy shift of 0.925 eV was added to all independent-particle transition energies in order to account for the underestimation of the band gap in DFT. This value was obtained in previous first-principles calculations on the level of the  $GW$  approximation [21]. Finally, we solve the Bethe-Salpeter equation iteratively for the first 2000 excitonic eigenenergies and envelope wave functions using the `SLEPc` library [36].

For the screened electron-phonon coupling, we approximate the two-particle interaction kernel on the level of time-dependent density functional theory. Lastly, for the phonon frequencies of the degenerate, Raman-active in-plane optical mode of  $E'$ -symmetry and the non-degenerate out-of-plane mode of  $A'_1$ -symmetry, we use the previously calculated values of  $391.7 \text{ cm}^{-1}$  and  $410.3 \text{ cm}^{-1}$  [32].

## Excitonic envelope wave functions

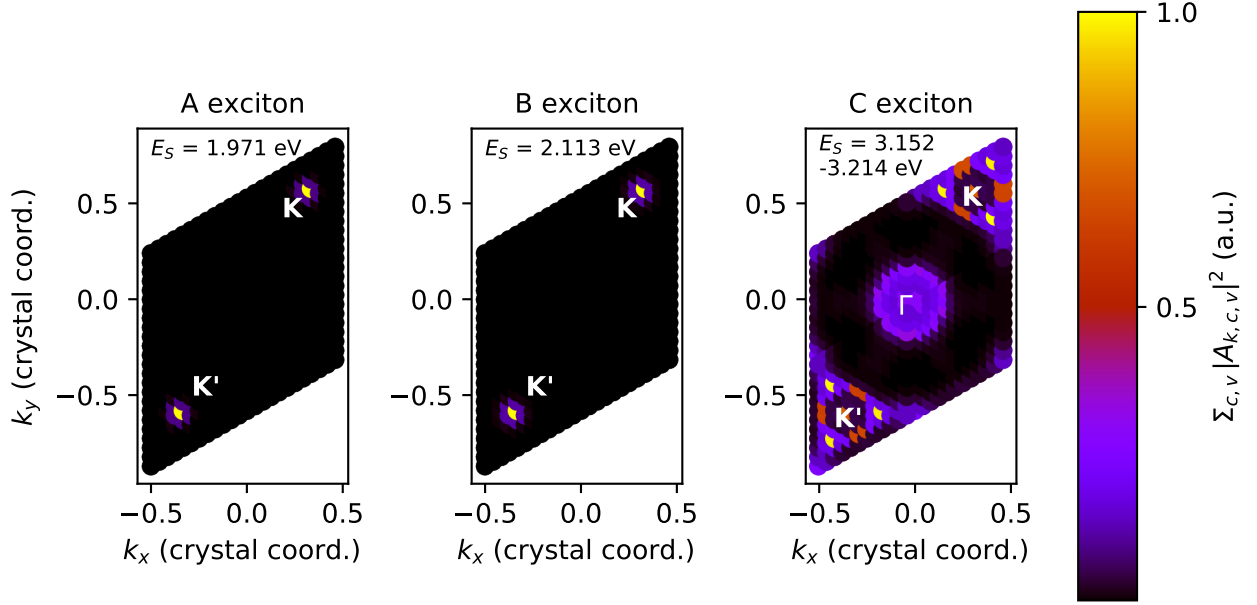

FIG. S6. **MoS<sub>2</sub>: Exciton envelope wave functions in reciprocal space.** Each panel shows the band-summed square of the envelope wave function  $|A_{\mathbf{k},c,v}^S|^2$  as a function of the wave vector  $\mathbf{k}$ . Shown are the wave functions of the first three bright excitons (the “A”-, “B”-, and “C”-excitons). In the case of the “C”-exciton, we show the sum of the squared wave functions of five energetically close bright excitons.

In Fig. S6, we show the state-summed envelope wave functions for the first three bright excitons, the so-called “A”-, “B”-, and “C”-excitons, as a function of wave vector  $\mathbf{k}$ . Both the “A”- and “B”-exciton are strongly localized around the  $K$ - and  $K'$ -point. In band space, they are dominated by transitions from the valence band bottom to the conduction band top, with the spin-orbit splitting of the valence band corresponding to the energy difference of the “A”- and “B”-exciton. By contrast, the “C”-exciton is considered to consist of a superposition of five bright and energetically close excitons [31]. It can no longer be attributed to a single, localized transition, but instead receives contributions from across large parts of the first Brillouin zone. As in the case of hBN, the circularly symmetric shape of the envelope wave functions of the “A”- and “B”-excitons means that in the corresponding energy regime, Raman scattering involving the degenerate in-plane  $E'$ -mode is suppressed due to angular momentum conservation [6, 13, 29]. By contrast, Raman scattering involving the  $A'_1$ -mode is still allowed as the latter does not carry any angular momentum. For the “C”-exciton, by contrast, the envelope wave function is strongly trigonally warped and hence both Raman modes are visible in the Raman spectrum.

## Electronic band structure

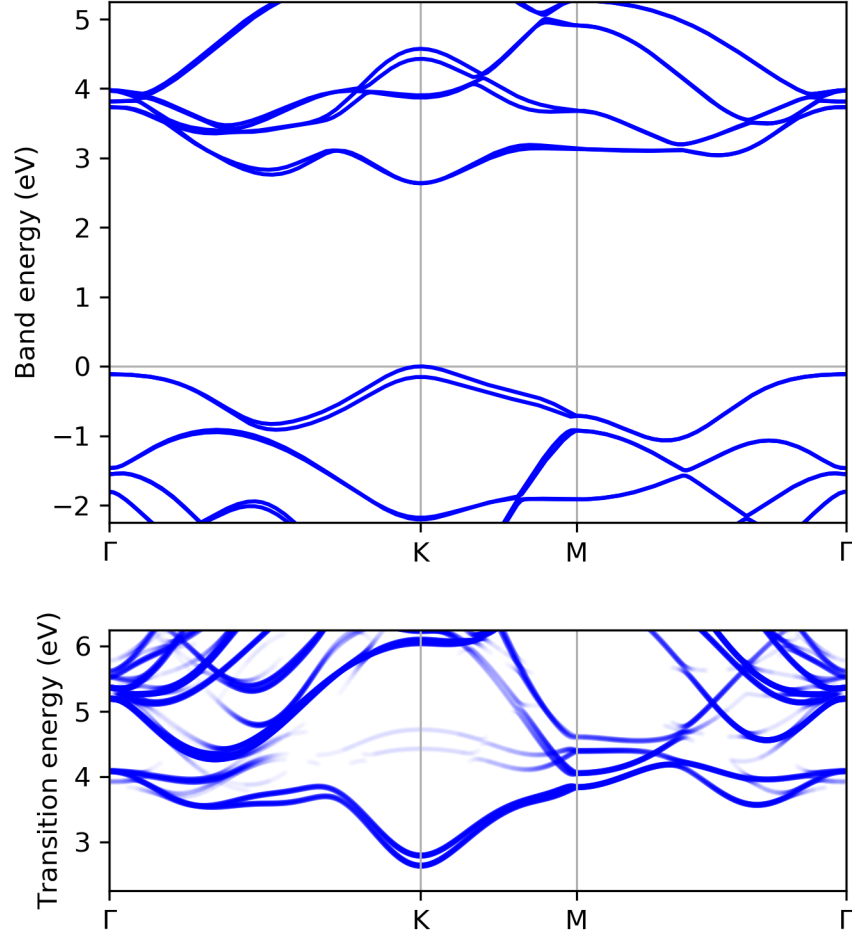

FIG. S7. **MoS<sub>2</sub>: Electronic (transition) band structure.** Top: Electronic band structure on the level of Kohn-Sham DFT within the LDA. A rigid shift of 0.925 eV was added to all conduction band energies. Bottom: Electronic transition band structure obtained from the electronic band structure. The opacity of the lines corresponds to the optical activity of the transition.

The electronic band structure of monolayer molybdenum disulfide is shown in Fig. S7. Again we show both the electronic band structure on the level of Kohn-Sham density functional theory on the LDA level (top panel) and the resulting transition band structure (bottom panel). As mentioned in the previous section, we shifted all conduction bands by 0.925 eV to account for the underestimation of the band gap in DFT [21].

The band structure is characterized by a direct gap of 2.633 eV at the  $K$ -point. The top of the valence band features a spin-orbit coupling-induced splitting of 0.112 eV, as its orbital decomposition involves Mo  $d$ -orbitals with finite angular momentum in  $z$ -direction, i.e., in the direction of the spin. By contrast, the conduction band bottom features a much smaller spin-orbit coupling-induced splitting of 0.003 eV, as it is mostly composed of Mo  $d$ -orbitals with zero angular momentum in  $z$ -direction. As a result the low-energy transition band structure consists of two almost degenerate doublets of transitions, separated by the valence band spin-orbit coupling-induced splitting. Due to the strong spin-orbit coupling, each member of the almost degenerate doublet is spin polarized. As a result, only one member of each doublet is optically active as a photon cannot flip the spin.

Finally, and as in hBN, the transition band structure around  $K^{(\prime)}$  is fully rotationally symmetric. This is important for the physics of Raman scattering involving the lowest two excitons, which receive finite contributions only from the region around  $K^{(\prime)}$ . As mentioned in the main text, this suppresses Raman scattering involving a finite-angular momentum phonon, as in the case of the  $E'$ -mode, in the low-energy regime (compare also the case of MoTe<sub>2</sub> [6]).

Raman intensity with only inter- or intra-exciton scattering

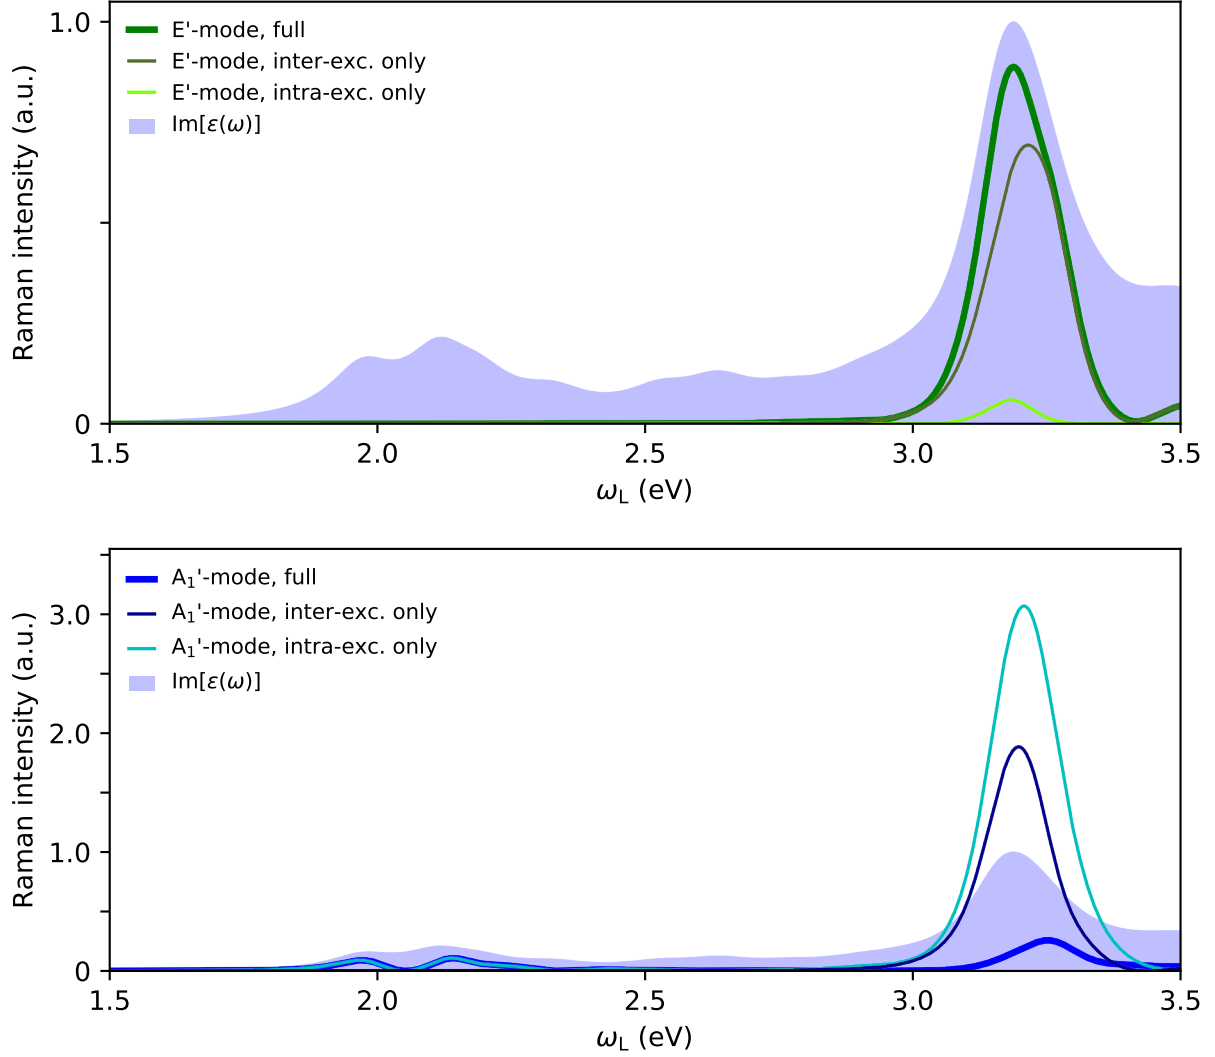

FIG. S8. **MoS<sub>2</sub>: Raman intensity with only inter- or intra-exciton scattering.** Raman intensity with all contributions (thick lines) and with only inter- or intra-exciton scattering (darker and lighter thin lines, respectively) taken into account. Top panel:  $E'$ -mode. Bottom panel:  $A_1'$ -mode. The shaded area represents the absorption spectrum. The Raman intensity is given in the same units in both panels and as in Fig. 3 of the main text.

As for the case of hBN, we examine the influence of intra- and inter-exciton scattering on the Raman intensity. In Fig. S8, we show the Raman intensity with only one of the two contributions for both the  $E'$ -mode (top panel) and the  $A_1'$ -mode (bottom mode). We only show the results for the non-adiabatic theory, as the adiabatic limit yields almost the same results, as mentioned in the main text.

Firstly, we note that in case of the  $E'$ -mode, the Raman intensity is strongly suppressed around the “A”- and “B”-excitons, irrespective of whether only intra- or inter-exciton scattering is considered alone. This further underlines that the suppression is indeed the result of a physical symmetry, i.e., in this case approximate full angular momentum conservation. Secondly, the Raman intensity for the  $E'$ -mode in the energy regime close to the “C”-exciton is dominated inter-exciton scattering and intra-exciton scattering plays almost no role.

In the case of the  $A_1'$ -mode, the picture is entirely different, however. The low-energy regime around the “A”- and “B”-excitons is governed by intra-exciton scattering due to the isolated nature of the two excitons. At higher excitation energies, inter-exciton scattering gains in weight and becomes almost as important as intra-exciton processes. Most

importantly though is the fact that the two scattering mechanism contribute to the total Raman matrix element with opposite signs. As such, the lower intensity of the  $A_1'$ -mode compared to that of the  $E'$ -mode is the effect of destructive quantum interference.

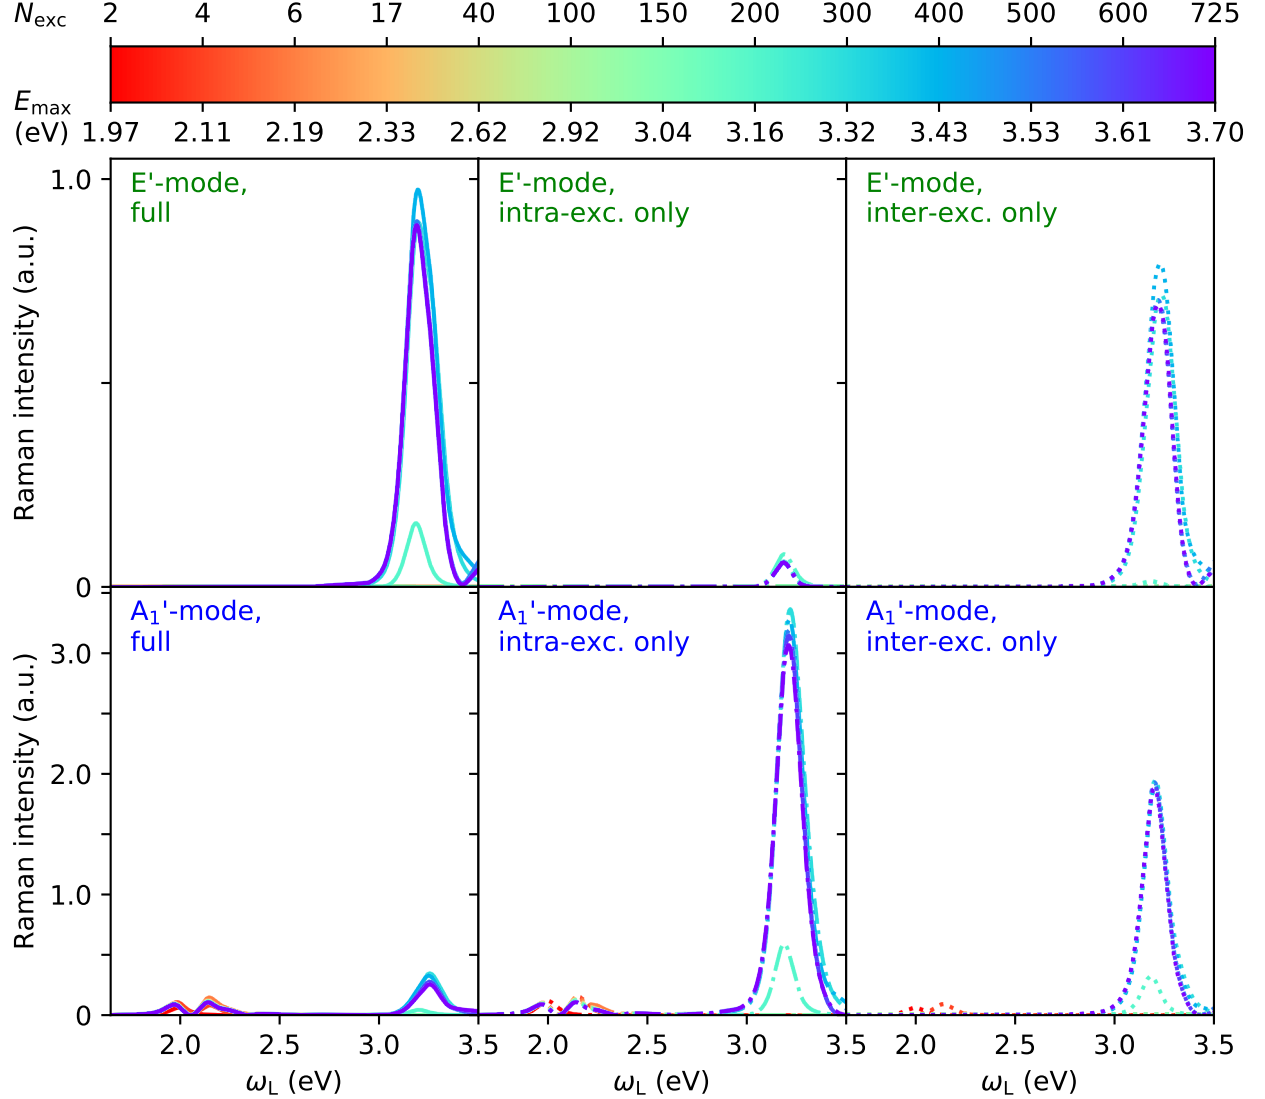

FIG. S9. **MoS<sub>2</sub>: Raman intensity for different numbers of exciton multiplets included.** Raman intensity for the  $E'$ -mode (top row) and for the  $A_1'$ -mode (bottom row) for different numbers of included exciton multiplets. The line color corresponds to the number of included exciton multiplets, with the maximum exciton energy included being indicated below the color bar. The three columns correspond to the Raman intensity with all contributions (left) and with only intra- (center) or inter-exciton (right column) scattering taken into account. The Raman intensity is given in the same units in all the panels and as in Fig. 3 of the main text.

Lastly, we briefly discuss the convergence of the inter-exciton contribution to the Raman intensity with the number of considered exciton multiplets  $N_{\text{exc}}$ , as the convergence behavior is different compared to the case of hBN. Since the frequency region around the “A”- and “B”-excitons is entirely dominated by intra-exciton scattering, we focus on the region around the “C”-exciton. From the right column of Fig. S9, it can be seen that the inter-exciton scattering part is already converged as soon as all the excitonic resonances that make up the “C”-exciton are included. This is different from the case of hBN, where the inter-exciton contribution still received sizable contributions from higher-energetic excitons. The reason for this different behavior can be attributed to the fact that the optically active excitons in the vicinity of the “C”-excitonic resonance are almost degenerate. As a results, their contribution to the inter-exciton part of the matrix element will be almost double-resonant, since it is proportional to  $[(\hbar\omega_L - E_S + i\gamma)(\hbar\omega_D - E_{S'} + i\gamma)]^{-1}$  with  $E_S \approx E_{S'}$ . By contrast, the contribution of higher-energetic excitons will only be single-resonant and thus

subdominant. In the case of hBN, however, the optically active excitons are well-separated in energy and their contributions can all only be single-resonant, which then requires the inclusion of a large number of excitons to reach convergence.
